# Supplementary material for: LatentKeypointGAN: Controlling Images via Latent Keypoints
Source: arXiv:2103.15812 source file (2024-10-13)
Supplement: Supplementary file 1 [file supp_editing.tex]

\section{More Editing} \label{sec:more_comparison}

\begin{figure*}
\begin{center}
\includegraphics[width=0.98\linewidth]{images/more_editing/integral_0.jpg}
\end{center}
   \caption{\textbf{Editing on FFHQ.} \textbf{The 1st column}: original image; \textbf{the 2nd column}: part appearance source image used to swap part appearance; \textbf{the 3rd column}: the combined image with shape from the original images and the appearance from the part appearance source image; \textbf{the 4th column}: only changing eyes; \textbf{the 5th column}: only changing mouth; \textbf{the 6th column}: only changing nose; \textbf{the 7th column}: scaling the face 0.85x down; \textbf{the 8th column}: scaling the face 1.15x up; \textbf{the 9th column}: move eyes closer; \textbf{the 10th column}: move eyes farther; \textbf{the 11th column}: move the face to the left and add another one on the right; 
   }
\label{fig:more_editing}
\end{figure*}

\begin{figure*}
\begin{center}
\includegraphics[width=0.98\linewidth]{images/more_editing/integral_15.jpg}
\end{center}
   \caption{\textbf{Editing.} 
   }
  \label{fig:more_editing2}
\end{figure*}

\begin{figure*}
\begin{center}
\includegraphics[width=0.98\linewidth]{images/more_editing/integral_30.jpg}
\end{center}
   \caption{\textbf{Editing.} 
   }
   \label{fig:more_editing3}
\end{figure*}

\begin{figure*}
\begin{center}
\includegraphics[width=0.98\linewidth]{images/more_editing/integral_45.jpg}
\end{center}
   \caption{\textbf{Editing.} 
   }
   \label{fig:more_editing4}
\end{figure*}

\begin{figure*}
\begin{center}
\includegraphics[width=0.98\linewidth]{images/more_editing/integral_60.jpg}
\end{center}
   \caption{\textbf{Editing.} 
   }
   \label{fig:more_editing5}
\end{figure*}

\begin{figure*}
\begin{center}
\includegraphics[width=0.98\linewidth]{images/more_editing/integral_75.jpg}
\end{center}
   \caption{\textbf{Editing.} 
   }
   \label{fig:more_editing6}
\end{figure*}

\begin{figure*}
\begin{center}
\includegraphics[width=0.98\linewidth]{images/more_editing/integral_90.jpg}
\end{center}
   \caption{\textbf{Editing.} 
   }
   \label{fig:more_editing7}
\end{figure*}

\begin{figure*}
\begin{center}
\includegraphics[width=0.98\linewidth]{images/more_editing/removing_0.jpg}
\end{center}
   \caption{\textbf{Removing keypoints one by one.} We remove the keypoints one by one for faces in Figure~\ref{fig:more_editing}. The first column shows the original image without removing any keypoints.
   }
\label{fig:removing}
\end{figure*}

\begin{figure*}
\begin{center}
\includegraphics[width=0.98\linewidth]{images/more_editing/removing_15.jpg}
\end{center}
   \caption{\textbf{Removing keypoints one by one.} We remove the keypoints one by one for faces in Figure~\ref{fig:more_editing2}.
   }
\end{figure*}

% \begin{figure*}
% \begin{center}
% \includegraphics[width=0.98\linewidth]{images/more_editing/removing_30.jpg}
% \end{center}
%   \caption{\textbf{Removing keypoints one by one.} We remove the keypoints one by one for faces in Figure~\ref{fig:more_editing3}.
%   }
% \end{figure*}

% \begin{figure*}
% \begin{center}
% \includegraphics[width=0.98\linewidth]{images/more_editing/removing_45.jpg}
% \end{center}
%   \caption{\textbf{Removing keypoints one by one.} We remove the keypoints one by one for faces in Figure~\ref{fig:more_editing4}.
%   }
% \end{figure*}

%----------------------------------------eye interpolation--------------------------------------

\begin{figure*}
\begin{center}
\includegraphics[width=0.98\linewidth]{images/more_editing/eyes_0.jpg}
\end{center}
   \caption{\textbf{Keypoint appearance embedding interpolation.} We show the interpolation of eyes for faces in Figure~\ref{fig:more_editing}. \textbf{The 1st column}: original image; \textbf{the 2rd-8th column}: the interpolation from the original images to the part source images; \textbf{the 9th column}: part appearance source image used to swap part appearance;; \textbf{the 10th column}: the difference between the original images and the swapped images.
   }
\label{fig:eye_interpolation}
\end{figure*}

\begin{figure*}
\begin{center}
\includegraphics[width=0.98\linewidth]{images/more_editing/eyes_15.jpg}
\end{center}
   \caption{\textbf{Keypoint appearance embedding interpolation.} We show the interpolation of eyes for faces in Figure~\ref{fig:more_editing}. \textbf{The 1st column}: original image; \textbf{the 2rd-8th column}: the interpolation from the original images to the part source images; \textbf{the 9th column}: part appearance source image used to swap part appearance;; \textbf{the 10th column}: the difference between the original images and the swapped images.
   }
\end{figure*}

\begin{figure*}
\begin{center}
\includegraphics[width=0.98\linewidth]{images/more_editing/eyes_30.jpg}
\end{center}
   \caption{\textbf{Keypoint appearance embedding interpolation.} We show the interpolation of eyes for faces in Figure~\ref{fig:more_editing2}.
   }
\end{figure*}

\begin{figure*}
\begin{center}
\includegraphics[width=0.98\linewidth]{images/more_editing/eyes_45.jpg}
\end{center}
   \caption{\textbf{Keypoint appearance embedding interpolation.} We show the interpolation of eyes for faces in Figure~\ref{fig:more_editing3}.
   }
\end{figure*}

%----------------------------------------mouth interpolation--------------------------------------

\begin{figure*}
\begin{center}
\includegraphics[width=0.98\linewidth]{images/more_editing/mouth_0.jpg}
\end{center}
   \caption{\textbf{Keypoint appearance embedding interpolation.} We show the interpolation of mouths for faces in Figure~\ref{fig:more_editing}. \textbf{The 1st column}: original image; \textbf{the 2rd-8th column}: the interpolation from the original images to the part source images; \textbf{the 9th column}: part appearance source image used to swap part appearance; \textbf{the 10th column}: the difference between the original images and the swapped images.
   }
\label{fig:mouth_interpolation}
\end{figure*}

\begin{figure*}
\begin{center}
\includegraphics[width=0.98\linewidth]{images/more_editing/mouth_15.jpg}
\end{center}
   \caption{\textbf{Keypoint appearance embedding interpolation.} We show the interpolation of mouths for faces in Figure~\ref{fig:more_editing1}.
   }
\end{figure*}

\begin{figure*}
\begin{center}
\includegraphics[width=0.98\linewidth]{images/more_editing/mouth_30.jpg}
\end{center}
   \caption{\textbf{Keypoint appearance embedding interpolation.} We show the interpolation of mouths for faces in Figure~\ref{fig:more_editing2}.
   }
\end{figure*}

\begin{figure*}
\begin{center}
\includegraphics[width=0.98\linewidth]{images/more_editing/mouth_45.jpg}
\end{center}
   \caption{\textbf{Keypoint appearance embedding interpolation.} We show the interpolation of mouths for faces in Figure~\ref{fig:more_editing3}.
   }
\end{figure*}

%----------------------------------------nose interpolation--------------------------------------

\begin{figure*}
\begin{center}
\includegraphics[width=0.98\linewidth]{images/more_editing/nose_0.jpg}
\end{center}
   \caption{\textbf{Keypoint appearance embedding interpolation.} We show the interpolation of noses for faces in Figure~\ref{fig:more_editing}. \textbf{The 1st column}: original image; \textbf{the 2rd-8th column}: the interpolation from the original images to the part source images; \textbf{the 9th column}: part appearance source image used to swap part appearance;; \textbf{the 10th column}: the difference between the original images and the swapped images.
   }
\label{fig:nose_interpolation}
\end{figure*}

\begin{figure*}
\begin{center}
\includegraphics[width=0.98\linewidth]{images/more_editing/nose_15.jpg}
\end{center}
   \caption{\textbf{Keypoint appearance embedding interpolation.} We show the interpolation of noses for faces in Figure~\ref{fig:more_editing2}.
   }
\end{figure*}

\begin{figure*}
\begin{center}
\includegraphics[width=0.98\linewidth]{images/more_editing/nose_30.jpg}
\end{center}
   \caption{\textbf{Keypoint appearance embedding interpolation.} We show the interpolation of noses for faces in Figure~\ref{fig:more_editing3}.
   }
\end{figure*}

\begin{figure*}
\begin{center}
\includegraphics[width=0.98\linewidth]{images/more_editing/nose_45.jpg}
\end{center}
   \caption{\textbf{Keypoint appearance embedding interpolation.} We show the interpolation of noses for faces in Figure~\ref{fig:more_editing4}.
   }
\end{figure*}

%----------------------------------------BBCPose-------------------------------------------
\begin{figure*}
\begin{center}
\includegraphics[width=0.98\linewidth]{images/more_editing/bbcpose_0.jpg}
\end{center}
   \caption{\textbf{Editing on BBCPose}. 
   }
\end{figure*}

%----------------------------------------Bedroom-------------------------------------------
\begin{figure*}
\begin{center}
\includegraphics[width=0.98\linewidth]{images/more_editing/bedroom_0.jpg}
\end{center}
   \caption{\textbf{Editing on LSUN Bedroom} \textbf{The 1st column}: original image; \textbf{the 2rd column}: part source images; \textbf{the 3th column}: swapping all parts; \textbf{the 4th column}: changing bed; \textbf{the 5th column}: removing bed.
   }
\end{figure*}

\begin{figure*}
\begin{center}
\includegraphics[width=0.98\linewidth]{images/more_editing/bedroom_30.jpg}
\end{center}
   \caption{\textbf{Editing on LSUN Bedroom}. 
   }
\end{figure*}

\begin{figure*}
\begin{center}
\includegraphics[width=0.98\linewidth]{images/more_editing/bedroom_failure_0.jpg}
\end{center}
   \caption{\textbf{Failure cases on LSUN Bedroom}. 
   }
\end{figure*}

%----------------------------------------comparison-------------------------------------------
\section{More Comparison with SEAN} \label{sec:more_comparison}
\begin{figure*}
\begin{center}
\includegraphics[width=0.98\linewidth]{images/more_editing/comparison_0.jpg}
\end{center}
   \caption{\textbf{Qualitative comparison with SEAN \cite{zhu2020sean}} The first five columns show our results and the last five columns show the results of SEAN \cite{zhu2020sean}. \textbf{Note that for SEAN, the first and the second columns are reconstructed image instead of edited images.} For two combined columns: \textbf{The 1st column}: original image; \textbf{the 2nd column}: part appearance source image used to swap appearance; \textbf{the 3rd column}: the combined image with shape from the original images and the appearance from the part appearance source image; \textbf{the 4th column}: only changing mouth \& jaw; \textbf{the 5th column}: only changing eyes.
   }
\label{fig:more_comparison}
\end{figure*}

\begin{figure*}
\begin{center}
\includegraphics[width=0.98\linewidth]{images/more_editing/comparison_15.jpg}
\end{center}
   \caption{\textbf{Qualitative comparison with SEAN \cite{zhu2020sean}}
   }
\end{figure*}

\begin{figure*}
\begin{center}
\includegraphics[width=0.98\linewidth]{images/more_editing/comparison_30.jpg}
\end{center}
   \caption{\textbf{Qualitative comparison with SEAN \cite{zhu2020sean}}
   }
\end{figure*}

\begin{figure*}
\begin{center}
\includegraphics[width=0.98\linewidth]{images/more_editing/comparison_45.jpg}
\end{center}
   \caption{\textbf{Qualitative comparison with SEAN \cite{zhu2020sean}}
   }
\end{figure*}

\begin{figure*}
\begin{center}
\includegraphics[width=0.98\linewidth]{images/more_editing/comparison_60.jpg}
\end{center}
   \caption{\textbf{Qualitative comparison with SEAN \cite{zhu2020sean}}
   }
\end{figure*}

\begin{figure*}
\begin{center}
\includegraphics[width=0.98\linewidth]{images/more_editing/comparison_75.jpg}
\end{center}
   \caption{\textbf{Qualitative comparison with SEAN \cite{zhu2020sean}}
   }
\end{figure*}

\begin{figure*}
\begin{center}
\includegraphics[width=0.98\linewidth]{images/more_editing/comparison_90.jpg}
\end{center}
   \caption{\textbf{Qualitative comparison with SEAN \cite{zhu2020sean}}
   }
\end{figure*}
